# Supplementary material for: Ultrafast Photodissociation Dynamics and Nonadiabatic Coupling Between Excited Electronic States of Methanol Probed by Time-Resolved Photoelectron Spectroscopy
Source: arXiv:1805.02648 source file (2018-10-30)
Supplement: Supplementary file 1 [file SI-Ultrafast_Photodissociation_Dynamics_and_Nonadiabatic_Coupling_Between_Excited_Electronic_States_of_Methanol_Probed_by_Time-Resolved_Photoelectron_Spectroscopy.pdf]

# Supporting Information for Ultrafast Photodissociation Dynamics and Nonadiabatic Coupling Between Excited Electronic States of Methanol Probed by Time-Resolved Photoelectron Spectroscopy

Elio G. Champenois,[1,2] Loren Greenman,[1,3,4] Niranjan Shivaram,[1] James P. Cryan,[5] Kirk A. Larsen,[1,2] Thomas N. Rescigno,[1] C. William McCurdy,[1,3] Ali Belkacem,[1] and Daniel S. Slaughter[1,a)]

[1)] *Chemical Sciences Division, Lawrence Berkeley National Laboratory, Berkeley, CA 94720, USA*

[2)] *Graduate Group in Applied Science and Technology, University of California, Berkeley, CA 94720, USA*

[3)] *Department of Chemistry, University of California, Davis, CA 95616, USA*

[4)] *Department of Physics, Kansas State University, Manhattan, KS 66506, USA*

[5)] *Stanford PULSE Institute, SLAC National Accelerator Laboratory, Menlo Park, CA 94025, USA*

(Dated: 30 October 2018)

[a)] DSSlaughter@lbl.gov

TABLE S1. Comparison of calculated excitation energies (in eV) with measurements and calculations of Cheng *et al.*[2].

| Excited state | $1^1A''$ | $2^1A''$ | $2^1A'$ | $3^1A'$ |
|---|---|---|---|---|
| Present calculations | 6.89 | 8.09 | 8.60 | 8.86 |
| Measured[2] | 6.76 | 7.72 | - | 8.3 |
| Calculated[2] | 6.6∼ 7.0 | 7.7∼ 8.2 | 8.3∼8.8 | 8.6∼9.4 |

## S1. CALCULATIONS OF THE POTENTIAL ENERGIES OF EXCITED ELECTRONIC STATES IN METHANOL

Satisfactory performance of the computational approach was determined by comparison of the calculated ionization potential of 11.0 eV with the measured value (10.846 eV±0.002 eV) of Macneil and Dixon[1] and calculated excitation energies with spectroscopic measurements of Cheng *et al.*[2], as listed in Table S1. The potential energy surfaces of methanol were explored in two degrees of freedom, the C–O–H angle, and the methyl C-H bond distance. The surface cuts (Figs S1-S5) were obtained by optimizing the geometry on the cation surface, using an approximate method for the geometry optimization (CASPT2). Potential energy calculations were then performed at the optimal points using EOM-CCSD. Both methods employed the aug-cc-pVTZ basis set.

Further exploring the process with a slower decay time and longer onset time of the C–H dissociation channel, a reaction coordinate was defined, linearly interpolating between the equilibrium geometries of the ground state of methanol and the $CH_2OH^+$ fragment, shown in Fig. S6. On the $S_3$ PES, there is a flat region as the in-plane C–H bond is stretched past 2.0 Å. It should be noted that there are many conformational changes occuring along this path, not just the C–H stretch. In fact, selective optimization of internal coordinates approximately orthogonal to the linear path between methanol and the fragment shows that there may be a shallow minimum in this region. Along this flat section of the PES, the probe pulse can ionize the fragmenting methanol even at large C–H bond distances, resulting in low kinetic energy electrons, as measured in the experiment (Figs 1 and 2). The delayed rise in the $CH_2OH^+$ signal (Fig. 4) can be attributed to the wavepacket motion that must first occur on $S_2$ before encountering the CI with $S_3$ where the fragmentation can take place. This

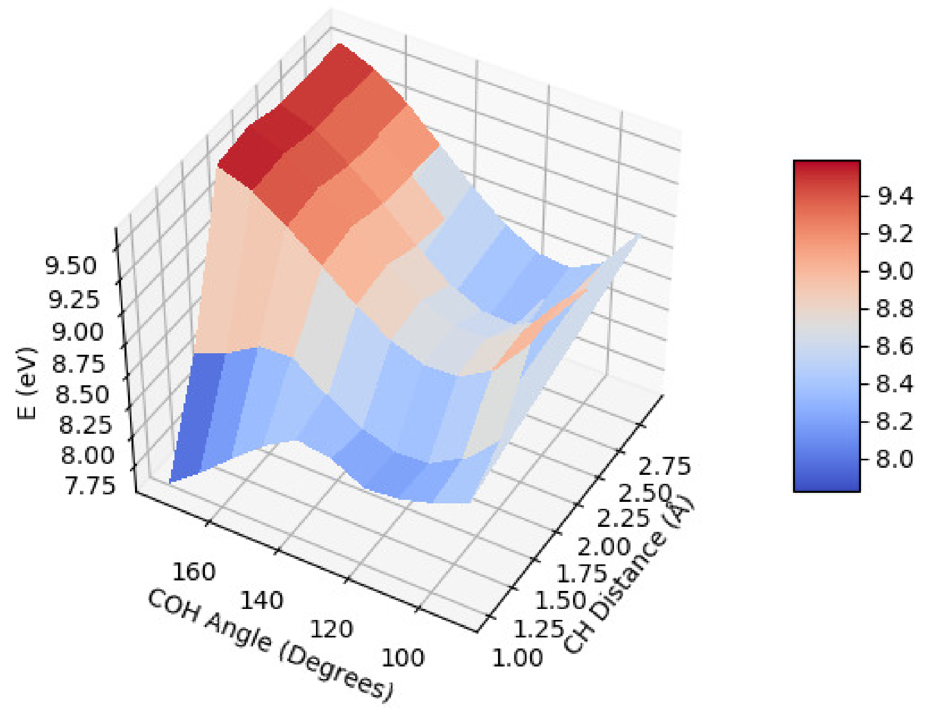


FIG. S1. 2-dimensional cut of the $S_2$ surface, for geometry optimized in the orthogonal degrees of freedom (DOFs) for the cation. The color scale is in eV.

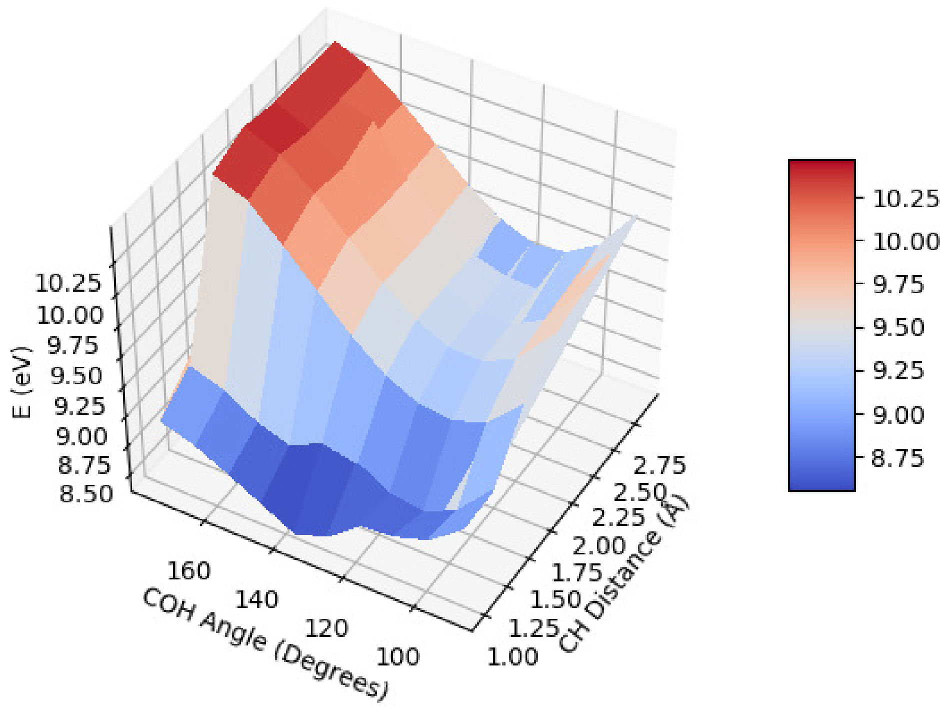


FIG. S2. 2-dimensional cut of the $S_3$ surface, for geometry optimized in the orthogonal DOFs for cation. The color scale is in eV.

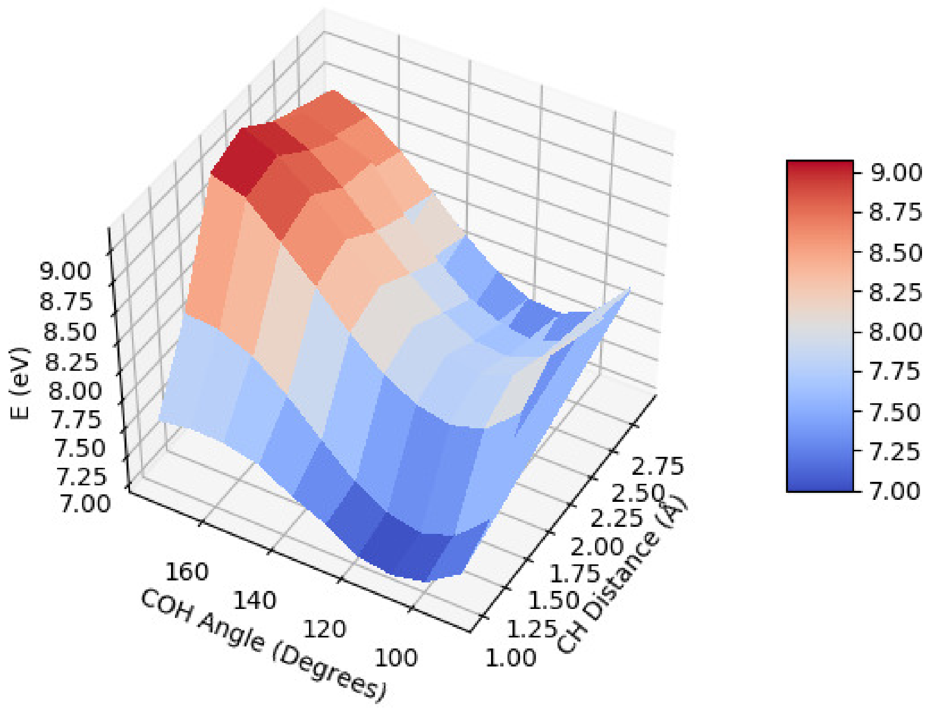


FIG. S3. $S_1$ surface, for geometry optimized in the orthogonal DOFs for the cation. The color scale is in eV.

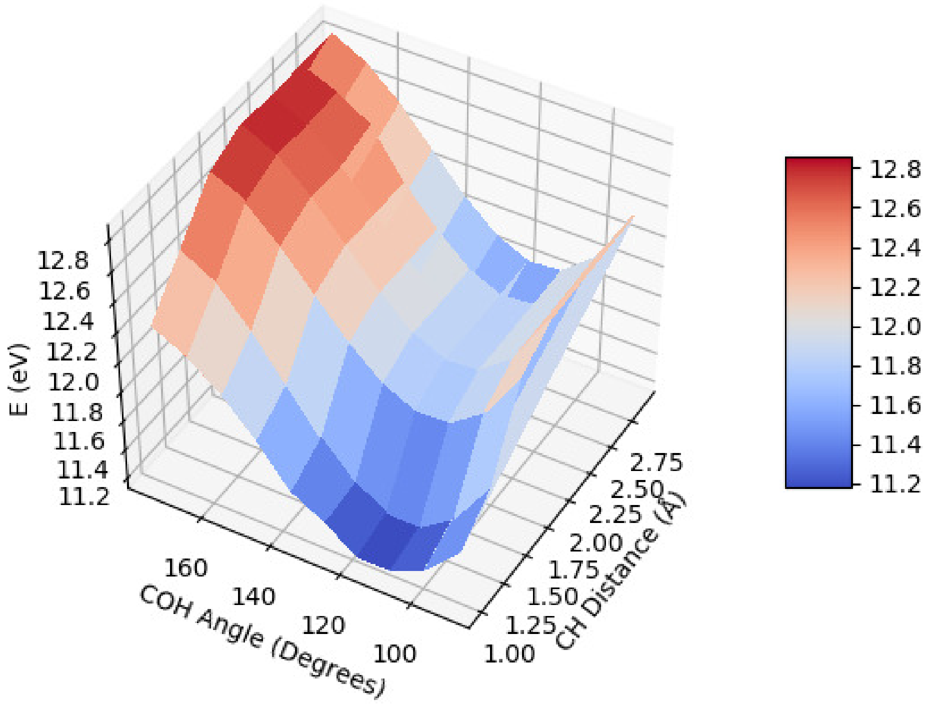


FIG. S4. 2-dimensional cut of the $D_0$ surface, for geometry optimized in the orthogonal DOFs for cation. The color scale is in eV.

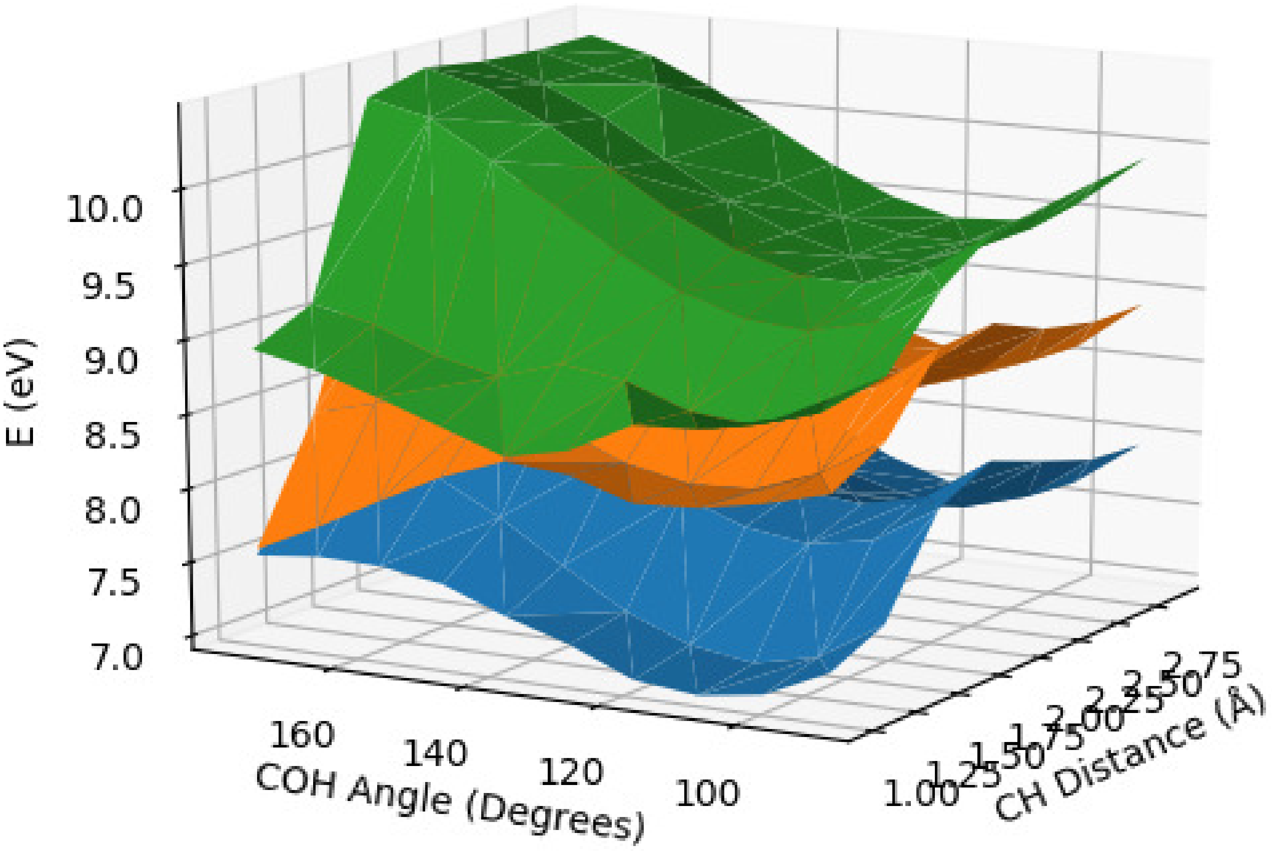


FIG. S5. 2-dimensional cut of the three lowest excited states of methanol $S_1$, $S_2$, $S_3$, for geometry optimized in the orthogonal DOFs for cation.

reaction mechanism also explains the strong effect of hydroxyl deuteration on the fragment lifetimes (Table 1) since it requires a significant opening of the C–O–H bond angle[3].

## S2. DETAILS OF THE FITTING PROCEDURE

Kinetic-energy slices of the photoelectron yield are plotted as a function of pump-probe delay in Fig. S7. The time shifts between successive slices are much finer than the width of the instrument response function (31.2 fs ± 0.9 fs) found in non-resonant ionization of xenon. A parameterized function, consisting of exponential decay and energy-dependent onset terms for the photoelectron yield, is used to fit the time-resolved photoelectron spectrum (TRPES) (Equation 2 in the main text). This model was selected due to its success in appropriately

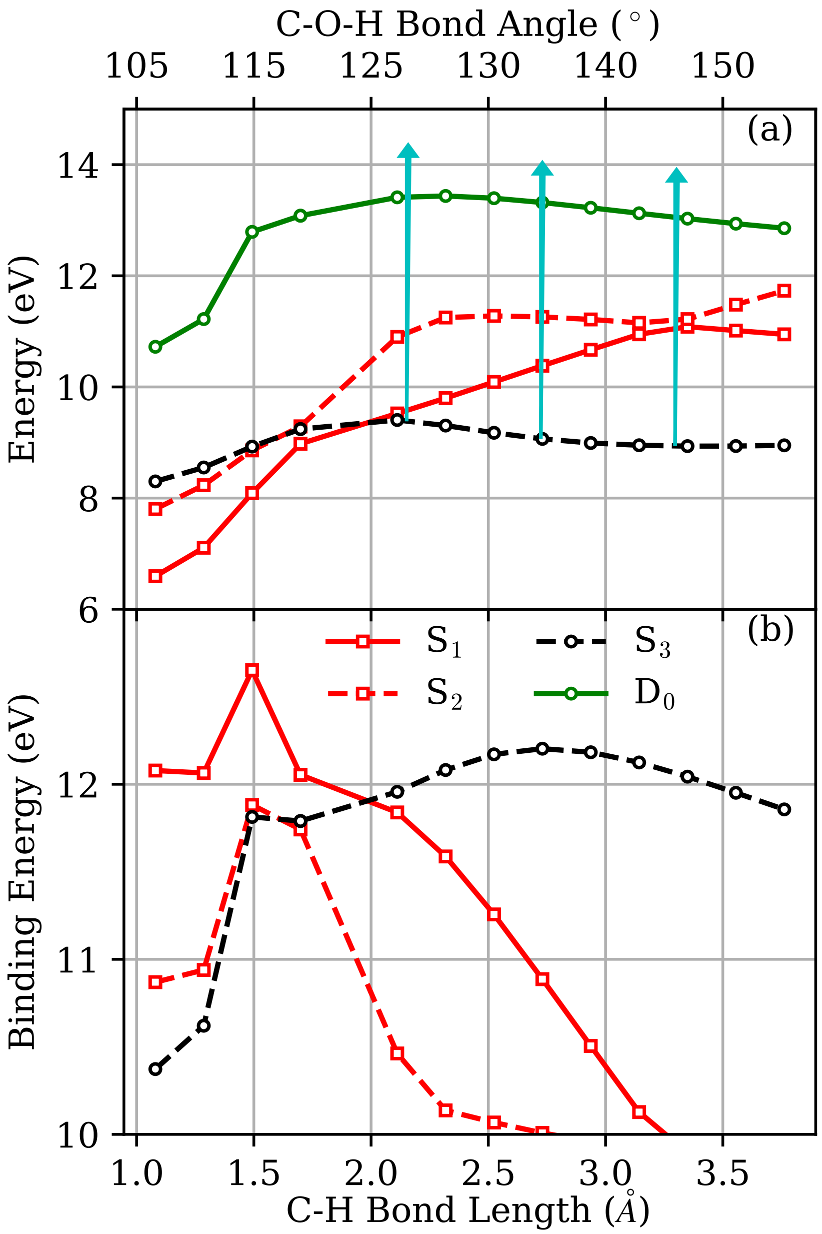


FIG. S6. Reaction pathway for the observed $CH_2OH^+$+H channel. The $S_1$, $S_2$, $S_3$ excited state, and $D_0$ cationic state (a) energies and (b) binding energies plotted as the C–H bond length and C–O–H bond angle. Beyond C–H stretch of 1.5 Å and C–O–H opening to 115°, the $S_3$ state binding energy is almost constant, allowing ionization of the system by a single probe photon (vertical arrows) for pump-probe time delays of up to 200 fs.

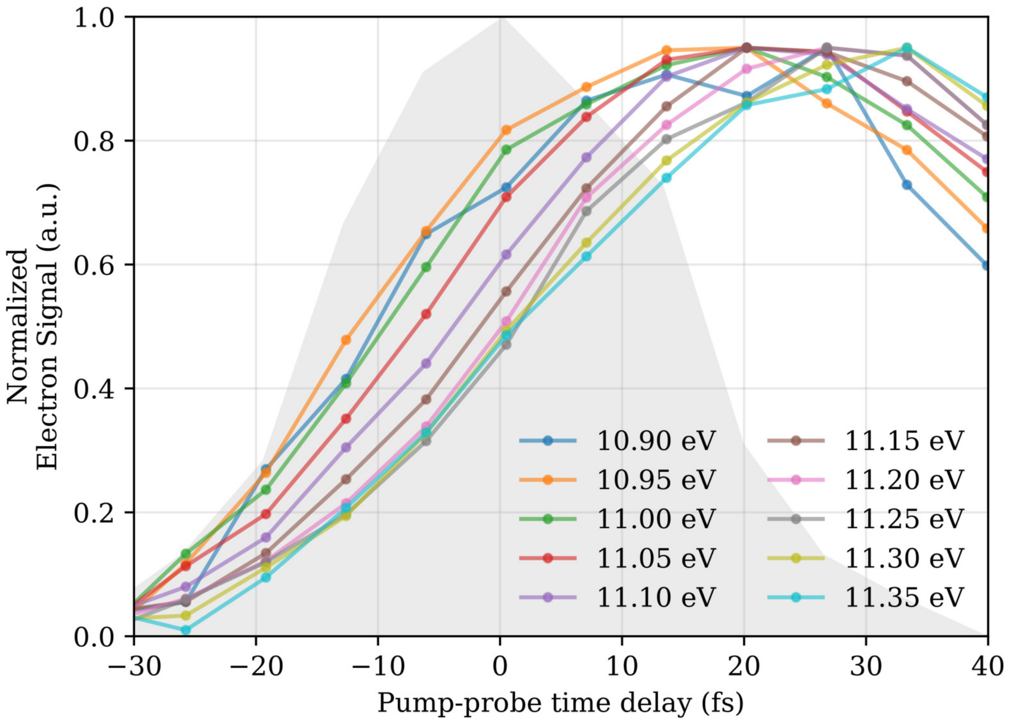


FIG. S7. Retrieved photoelectron signal onset times (red, left axis) and decay associated amplitudes (right axis) $A_1$ (blue) and $A_2$ (cyan). The two decay times extracted from the fit are $\tau_1$=25 fs and $\tau_2$=72 fs. $A_2$ is multiplied by a factor of four for increased visibility.

fitting the data and its ability to quantify both the energy-shifting and decay features. For comparison, a secondary fitting approach using global lifetime analysis of decay associated spectra (for example, see Townsend *et al.*[4]), modified to incorporate the energy-dependent signal onset times $t_0(\mathcal{E})$, was also performed and the results are shown in Fig. S8. Only N=2 lifetimes are needed for a good fit to the data using:

$$I(\mathcal{E},t) = \sum_{i}^{N} A_i(\mathcal{E}) \times \exp\left(-\frac{t - t_0(\mathcal{E})}{\tau_i(\mathcal{E})}\right) \otimes g(t - t_0(\mathcal{E}); \sigma), \tag{1}$$

where $A_i(\mathcal{E})$ are the decay associated amplitudes. Each model accounts for the major features in the measured TRPES, and facilitates the analysis of the transient binding energy of the photoexcited system. As expected, the signal onset times $t_0(\mathcal{E})$ found here are in good agreement with those found using the first model. The extracted Gaussian full-width-at-half maximum of 44.8 fs $\pm$ 0.5 fs is considerably broader than the instrument response function.

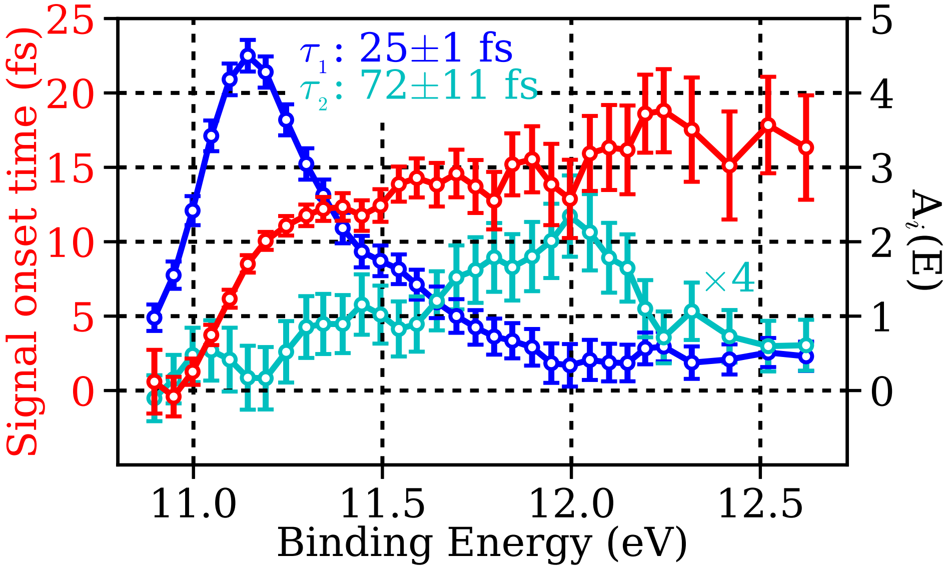


FIG. S8. Retrieved photoelectron signal onset times (red, left axis) and decay associated amplitudes (right axis) $A_1$ (blue) and $A_2$ (cyan). The two decay times extracted from the fit are $\tau_1$=25 fs and $\tau_2$=72 fs. $A_2$ is multiplied by a factor of four for increased visibility.

## SUPPLEMENTARY REFERENCES

[1] K. A. G. Macneil and R. N. Dixon, "High-resolution photoelectron spectroscopy of methanol and its deuterated derivatives: Internal rotation in the ground ionic state," Journal of Electron Spectroscopy and Related Phenomena **11**, 315–331 (1977).

[2] B.-M. Cheng, M. Bahou, W.-C. Chen, C.-h. Yui, Y.-P. Lee, and L. C. Lee, "Experimental and theoretical studies on vacuum ultraviolet absorption cross sections and photodissociation of $CH_3OH$, $CH_3OD$, $CD_3OH$, and $CD_3OD$," The Journal of Chemical Physics **117**, 1633–1640 (2002).

[3] T. Okino, Y. Furukawa, P. Liu, T. Ichikawa, R. Itakura, K. Hoshina, K. Yamanouchi, and H. Nakano, "Coincidence momentum imaging of ultrafast hydrogen migration in methanol and its isotopomers in intense laser fields," Chemical Physics Letters **423**, 220–224 (2006).

[4] D. Townsend, H. Satzger, T. Ejdrup, A. M. D. Lee, H. Stapelfeldt, and A. Stolow, "$^1B_2(^1\Sigma_u^+)$ excited state decay dynamics in $CS_2$," The Journal of Chemical Physics **125**, 234302 (2006).
